# Supplementary material for: How Long to Estimate Sparse MIMO Channels
Source: arXiv:2101.07287 source file (2021-01-18)
Supplement: Supplementary file 1 [file Appendix_I.tex]

\begin{proof}
Since $\boldsymbol{G}$ satisfies RIP of order $k$ with constant $\delta_k$, then by Lemma \ref{lemma:RIP_kronecker}, we have that both $\boldsymbol{M_t}$ and $\boldsymbol{M_r}$ satisfy RIP of order $k$ with constants $\delta_k^{(t)}$ and $\delta_k^{(r)}$, respectively, where
\begin{equation}
\max\left\lbrace \delta_k^{(t)}, \delta_k^{(r)} \right\rbrace \leq \delta_k.
\end{equation}
Also, by Lemma \ref{lemma:m*}, there exists a function $g(\cdot)$, that is non-increasing in $\delta_k^{(i)}$, which we can use to find asymptotic lower bounds on $m_t$ and $m_r$. Since $g(\cdot)$ is non-increasing in $\delta$, then
\begin{equation} \footnotesize
g\left(n_t; \delta_k^{(t)}, k\right) \geq g\left(n_t; \delta_k, k\right), \quad\quad g\left(n_r; \delta_k^{(r)}, k\right) \geq g\left(n_r; \delta_k, k\right)
\end{equation}
Thus, it follows that
\begin{align}
m_t &\in \Omega \left( g\left(n_t; \delta_k^{(t)}, k\right) \right) \subseteq \Omega \left( g\left(n_t; \delta_k, k\right) \right) \label{eq:thm:main:1} \\ 
m_r &\in \Omega \left( g\left(n_r; \delta_k^{(r)}, k\right) \right) \subseteq \Omega \left( g\left(n_r; \delta_k, k\right) \right) \label{eq:thm:main:2} 
\end{align}
Let $m$ denote the number of rows of $\boldsymbol{G}$. By construction, we have $m = m_t m_r$.
By Eq. (\ref{eq:thm:main:1}), $\exists \; c_1 > 0, n_1 \in \mathbb{N}^+$ such that $m_t \geq c_1 g\left(n_t; \delta_k, k\right)$ for all $n_t \geq n_1$. Similarly, by Eq. (\ref{eq:thm:main:2}), $\exists \; c_2 > 0, n_2 \in \mathbb{N}^+$ such that $m_r \geq c_2 g\left(n_r; \delta_k, k\right)$ for all $n_r \geq n_2$.
Thus, we have $m_t m_r \geq c_1 c_2 g\left(n_t; \delta_k, k\right) g\left(n_r; \delta_k, k\right)$ for all $n_t, n_r \geq n_3$, where $n_3 = \max \{n_1, n_2\}$.
Therefore, $m = \Omega\left( \left( g\left(n_t; \delta_k, k\right) g\left(n_r; \delta_k, k\right) \right) \right)$.
\end{proof}
%\begin{lemma}[RIP of the Kronecker Product \cite{jokar2009sparse, roth2018hierarchical}]\label{lemma:RIP_kronecker}
%The RIP constant $\delta_k\left(\cdot\right)$ of the Kronecker product of $J$ matrices $\boldsymbol{M_1}, \boldsymbol{M_2}, \dots, \boldsymbol{M_J}$, each with an RIP of order $k$ with constants $\delta_k^{(1)}, \delta_k^{(2)}, \dots, \delta_k^{(J)} $, respectively, is bounded as:
%\begin{equation}
%\footnotesize
%\max_{1 \leq j \leq J} \delta_k^{(j)}  \leq \delta_k \left( \boldsymbol{M_1} \otimes \boldsymbol{M_2} \otimes \dots \otimes \boldsymbol{M_J}\right) \leq \prod_{j = 1}^J \left( 1+\delta_k^{(j)} \right) -1
%\end{equation}
%\end{lemma}
