# Supplementary material for: How Long to Estimate Sparse MIMO Channels
Source: arXiv:2101.07287 source file (2021-01-18)
Supplement: Supplementary file 2 [file Appendix_II.tex]

\begin{proof}
Part \ref{thm:statement1} follows by Lemma \ref{lemma:RIP_kronecker} since $\boldsymbol{G_v}$ satisfies RIP of order $2k$ with constant $\delta$.
Now, let the RIP constants satisfied by $\small \left(\boldsymbol{F}^H \boldsymbol{U_t}\right)^{\ast}$ and $\small  \boldsymbol{W}^H \boldsymbol{U_r}$ be $\delta_{2k}^{(f)}$ and $\delta_{2k}^{(w)}$, respectively.
Then, by Theorem \ref{thm:davenPortBnd}, we have
$m_t \geq 2c_{\delta_{2k}^{(f)}}k \log \left( \frac{n_t}{2k} \right)$
and
$m_r \geq 2c_{\delta_{2k}^{(w)}}k \log \left( \frac{n_r}{2k} \right)$.
Next, observe that $c_{\delta}$, as defined in Theorem \ref{thm:davenPortBnd}, is a monotonically decreasing function in $\delta$ for $\delta\in\left(0,1\right)$ since $\frac{d c_{\delta}}{d \delta}$ is given by
\begin{equation}
\small
\frac{d c_{\delta}}{d \delta} = \frac{- \frac{1}{2} \left(1 + \sqrt{\frac{1+\delta}{1-\delta}}\right) \left( \frac{1}{(1-\delta) \sqrt{(1+\delta)(1-\delta)}} \right)}{\log^2\left(\sqrt{\frac{1+\delta}{1-\delta}} +1\right)} < 0
\end{equation}
Therefore, we have
\small{
\begin{align}
m_t &\geq 2 c_{\delta_{2k}^f} k \log \left( \frac{n_t}{2k} \right) \geq 2 c_{\delta} k \log \left( \frac{n_t}{2k} \right) \label{eq:mt_bound} \\
m_r &\geq 2 c_{\delta_{2k}^w} k \log \left( \frac{n_r}{2k} \right) \geq 2 c_{\delta} k \log \left( \frac{n_r}{2k} \right) \label{eq:mr_bound},
\end{align}}%
\normalsize
which proves part \ref{thm:statement2}.\\
Finally, since $c_{\delta} > 0$, we get part \ref{thm:statement3} by multiplying the lower bounds of $m_t$ and $m_r$.
\end{proof}
