# Supplementary material for: How Long to Estimate Sparse MIMO Channels
Source: arXiv:2101.07287 source file (2021-01-18)
Supplement: Supplementary file 3 [file Appendix_IV.tex]

\begin{proof}
%Recall that $n_t \geq k^{1+\epsilon}$ and $k$ grows with $n_t$ (by assumption, see Section \ref{sec:sysModel}).
%Then, there exist constants $c_1 \in \mathbb{R}^+$ and $N \in \mathbb{N}$ such that $\log \frac{n_t}{2k} \geq c_1 \log \frac{n_t}{k}$ for all $n_t \geq N$.
%Simply, put $c_1 = 1 - \log2 > 0$ and $N$ such that $\log \frac{N}{k} \geq 1$.
%Thus, we have that $m_t \geq 2 c_{\delta} c_1 k \log\left(\frac{n_t}{k}\right)$. Similarly, we choose a constant $c_2 \in \mathbb{R}^+$ such that $m_r \geq 2 c_{\delta} c_2 k \log\left(\frac{n_r}{k}\right)$.
%Therefore, we have that $m_t  = \Omega \left( k \log \frac{n_t}{k} \right)$ and $m_r  = \Omega \left( k \log \frac{n_r}{k} \right)$.
%Thus, by Theorem \ref{thm:main} it follows that $m = m_t m_r = \Omega \left( k^2 \log \left(\frac{n_t}{k}\right) \log \left( \frac{n_r}{k}\right) \right)$.
We will show that $\log \left( \frac{n_i}{2k} \right) \geq c_i  \log \left( \frac{n_i}{k} \right)$ for some constant $c_i > 0$ and $i \in \left\lbrace t, r \right\rbrace$.
Then, from Eq. (\ref{eq:statement3}), we shall have that $m \ge C k^2 \log\left(\frac{n_t}{k}\right) \log\left(\frac{n_r}{k}\right)$, where $C = 4 c_{\delta}^2 c_t c_r > 0$. Hence, Eq. (\ref{eq:mybound}) follows.\\
Now, set $c_i = 1 - \log2 > 0$. Then, we have that $\log \left( \frac{n_i}{2k} \right) \geq c_i  \log \left( \frac{n_i}{k} \right)$ for all $n_i$ such that $\log \frac{n_i}{k} \geq 1$.
Recall that $\frac{n_i}{k}$ increases as $n_i$ increases, for $i \in \left\lbrace t,r \right\rbrace$ (by assumption). Then, there exists $N_i \in \mathbb{N}$ such that $\log \frac{n_i}{k} \geq 1$ for all $n_i \geq N_i$.
\end{proof}
